# Supplementary material for: Site-site interaction model for alcohol models in two-dimensions
Source: arXiv:2409.14871 source file (2024-09-23)
Supplement: Supplementary file 1 [file SI.pdf]

# Supporting Information For Publication

## Site-site interaction model for alcohol models in two-dimensions

Aurélien Perera

Laboratoire de Physique Théorique de la Matière Condensée (UMR CNRS 7600), Sorbonne Université, 4 Place Jussieu, F75252, Paris cedex 05, France.

### 1) – Structure factors and other functions concerned with scattering intensity

Fig.S1 shows, for the pair of atoms $O$ and $C_n$ , where is the terminal atom of the alkyl chain – n=2 for ethanol and n=8 for octanol, the structure factor $S_{OC_n}(k)$ of Eq.(5), the total structure factor $S_{OC_n}^{(T)}(k)$ of Eq.(6), the intra-molecular correlation $w_{OC_n}(k)$ of Eq.(7) and the form factor $f(k)=f_O(k)=f_{C_n}(k)$ of Eq.(9) (which has been taken as the same for all atoms).

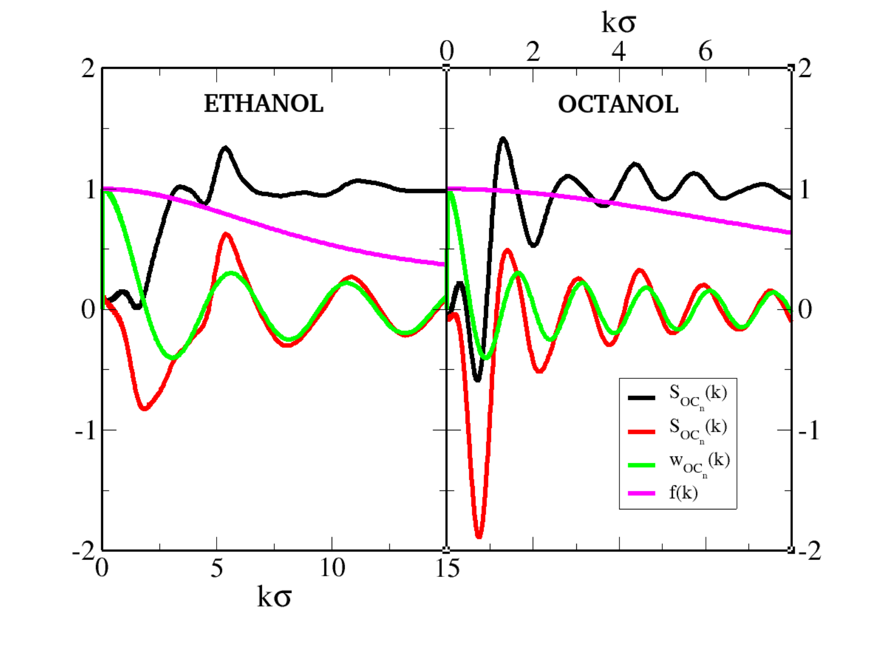


Fig.S1 – site-site structure factor, total structure factor, intra-molecular correlation function and form factor for ethanol ( $n=2$ ) in the left panel and octanol ( $n=8$ ) in the right panel, for the oxygen $O$ site and the terminal $C_n$ carbon site.

These functions serve also to illustrate the charged ( $O$ ) and uncharged ( $C_n$ ) site cross correlations, which produce negative pre-peak contributions to the scattering intensity $I(k)$ (Eq.8), as can be seen from the total structure factor $S_{OC_n}^{(T)}(k)$ . In addition, while the main peak in both figures is around $k\sigma\approx 6$ (as for a standard Lennard-Jones liquid), the pre-peaks are not at the same positions for ethanol and octanol. This is because the depletion distance between the O and C_n sites is smaller for ethanol than for octanol, resulting in pre-peaks at larger and smaller k values, respectively. It is equally seen that octanol has 2 pre-peaks, the inner one corresponding to the broken pile structure induced by the alkyl tail packing, which can be seen in the snapshot for octanol in the the upper right panel of Fig.5.

## 2 ) - Thermodynamic properties

Fig.S2 illustrates the density dependence of the total and Coulomb excess internal energy per particle and the compressibility factor for the temperature T=2, for ethanol and octanol.

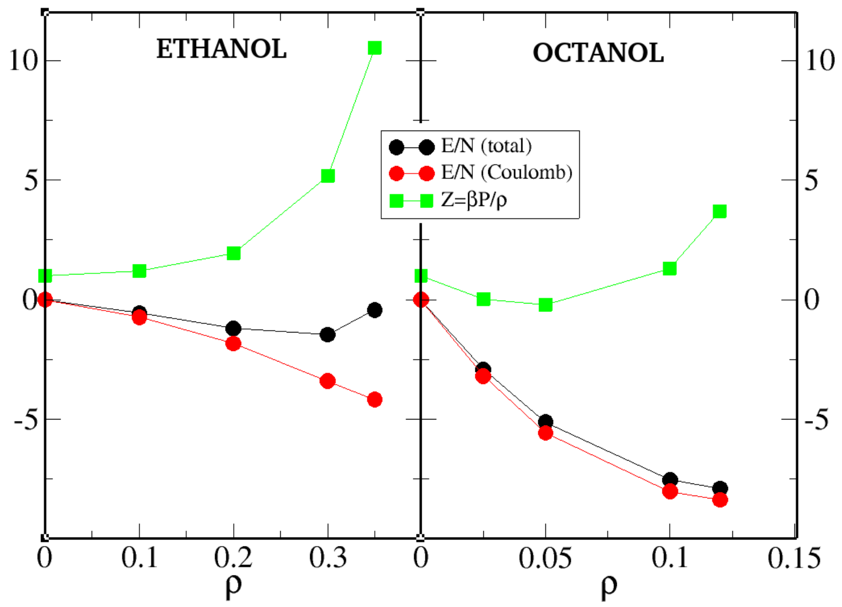


Fig.S2 – Density dependence of E/N (total and Coulomb) and Z for T=2 for ethanol (left panel) and octanol (right panel)

It is seen that the Coulomb interaction dominates the contributions to the total energy, except for the high density regime of ethanol, where temperature induced disorder can have a larger influence than for octanol, because of the tail packing effects. Indeed, it is more difficult to produce disorder in long tails which tend to pack parallel to each other, than in the case of the shorter 2 carbon tail, which can be rotated more freely. The tail induced ordering also tends to depress the pressures, as can be seen from the compressibility factors.
